# Supplementary material for: InstructAny2Pix: Flexible Visual Editing via Multimodal Instruction Following
Source: arXiv:2312.06738 source file (2024-10-17)
Supplement: Supplementary file 1 [file X_suppl.tex]

\clearpage
\setcounter{page}{1}
   {
   \newpage
       
        {\centering
        % \Large
        \textbf{Appendix}\\
        \vspace{0.5em}Appendix \\
        \vspace{1.0em}}
   }
\section{Details of Datasets}
We use SoundNet \cite{aytar2016soundnet}, VGG-Sound \cite{chen2020vggsound}, and AudioSet \cite{gemmeke2017audio} for audio-visual alignment. These datasets consist of videos with audio. We extract the audio and the middle frame from the video to create audio-image pairs. SoundNet consists of 802,724 audio-image pairs, AudioSet consists of 888,185 audio-image pairs, and VGG-Sound consists of 197,958 pairs. These numbers represent the number of valid video URLs at the time of data fetching (Oct 2023). They may differ from the original dataset size and the number of valid URLs at the time of writing. We also make use of audio captions from MusicCaps \cite{agostinelli2023musiclm} and AudioCaps \cite{audiocaps} to create text-audio pairs. These two datasets provide text captions for subsets of AudioSet. They do not introduce new audio files. We use LAION-Aesthetic-3M \cite{schuhmann2022laion} for text-image alignment, which consists of 2,209,745 valid image URLs at the time of data fetching (Sep 2023). All these datasets are used in our prior training.

\section{Implementation Details}

\subsection{MM-Inst Datasets}
\subsubsection{Source Captions}
We use BLIP2 \cite{li2023blip} to generate captions for 500,000 images randomly selected among 2,209,745 images from LAION-Aesthetic-3M. We use an off-the-shelf implementation and do not make any modifications from the default settings. This step is necessary because the original LAION caption contains many non-descriptive texts such as ``Wholesale high-quality painting POP art fish free shipping."

\subsubsection{Instruction Generation}
In the instruction generation phase, we consider the following atomic operations: add, drop, replace, style change, and atmosphere change. In particular, style change refers to changes in visual style, such as changing a realistic photo into a painting, 3D rendering, or anime. Atmosphere change refers to the overall ``mood" an image conveys, such as scary, disturbing, exciting, or peaceful. The concept of atmosphere is mostly used when fitting an image to music. We also consider a combination of multiple instructions. For each of the 500,000 image captions, we prompt LLAMA2 \cite{touvron2023llama} with the caption and examples of editing instructions. Since LLAMA2 does not have multi-modal capability, we provide descriptions of multi-modal input and prompt it to generate descriptions of multi-modal input as well. Table \ref{tab:generation_inst} lists examples of instructions from each category used for prompting. To ensure the diversity of instructions, we randomly select one or more atomic editing operations for each caption and explicitly prompt LLAMA2 to generate a simple instruction of the specified type or a composite instruction involving the specified types of atomic editing operations. Table \ref{tab:prompting} illustrates the overall prompting template for a given caption.

\begin{table}
    \centering
    \begin{tabular}{p{1cm}|p{3cm}|p{3cm}}
         Type & Example & Result \\
         \hline 
         Add & Please incorporate [an image of cannon fire] into [an image of a pirate ship sailing on the high sea] & An image of a pirate ship firing at a British Navy warship, fire burning on the ship \\
         \hline 
         Remove & Remove [sound of car accelerating] from [an image of people driving in the countryside road] & An image of a quiet countryside road \\
         \hline
         Replace & Replace [sound of dog barking] with [sound of a cute cat] for [an image of a dog at the beach] & An image of a cat at the beach \\
         \hline
         Style & Change [an image of a woman wearing sunglasses in Paris] to the style of [an image of a Renaissance painting of a noble lady] & A Renaissance painting of a woman wearing sunglasses in Paris \\
         \hline
         Atom. & Make [an image of a cute girl in a school uniform] fit the atmosphere of [a piece of music of stellar constellations] & An image of a cute girl in a school uniform under the night sky \\
         & \\
    \end{tabular}
    \caption{Examples of different types of instructions. Atom.: Atmosphere change.}
    \label{tab:generation_inst}
\end{table}

\begin{table}
    \centering
    \begin{tabular}{p{8cm}}
        Template:\\
        \hline
        I need to generate some multi-modal editing operations. Here are some examples:\\
        \textcolor{blue}{\text{[examples of instructions]}} \\
        In summary, operations include add, drop, replace subjects. Style transfer and fitting a coherent atmosphere.  \\
        Please generate following the example above. Given the base caption \text{\textcolor{blue}{[base caption]}}. (You should always use this base). \\
        I only need one example on \textcolor{blue}{\text{[type(s) of instruction]}}. Please stop after that. The output should follow the exact format as provided. This is very important!\\
        The editing should also be relevant to the original scene. It should not be random. For example, you should not try adding a rainbow to everything. This is very important!\\
        
    \end{tabular}
    \caption{Instruction generation prompt used to generate MM-Inst Dataset. Highlighted areas are replaced with corresponding data. Base caption refers to the caption of the edit target.}
    \label{tab:prompting}
\end{table}

\subsubsection{Multi-Modal Feature Generation}
For image features corresponding to source captions, we use the features extracted from respective images in the dataset. For additional image and audio features in the instruction, we use our prior model to generate these features from corresponding texts. For output image features, we additionally use features extracted from edited images generated by DDIM inversion. These features are used as inputs and outputs of LLM.

\begin{figure*}[t]
    \centering
    \includegraphics[width=490px]{assets/appendix1.pdf}
    \caption{Qualitative Results on MM-Inst Test Dataset. For convenience, we provide text descriptions of images and audios in brackets. At runtime, however, the model is not exposed to text descriptions of multi-modal inputs. We recommend zooming in for a better viewing experience.}
    \label{fig:additional_demo}
\end{figure*}
\begin{figure*}[t]
    \centering
    \includegraphics[width=490px]{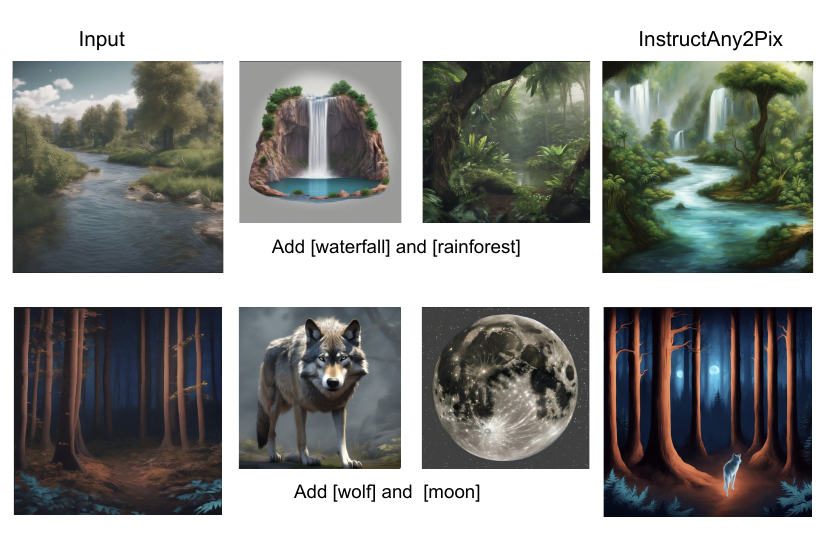}
    \caption{Qualitative Results on MM-Inst Test Dataset. In this figure, we demonstrate multi-image scene composition. For convenience, we provide text descriptions of images and audios in brackets. At runtime, however, the model is not exposed to text descriptions of multi-modal inputs. We recommend zooming in for a better viewing experience.}
    \label{fig:additional_demo_11}
\end{figure*}
\begin{figure*}[t]
    \centering
    \includegraphics[width=490px]{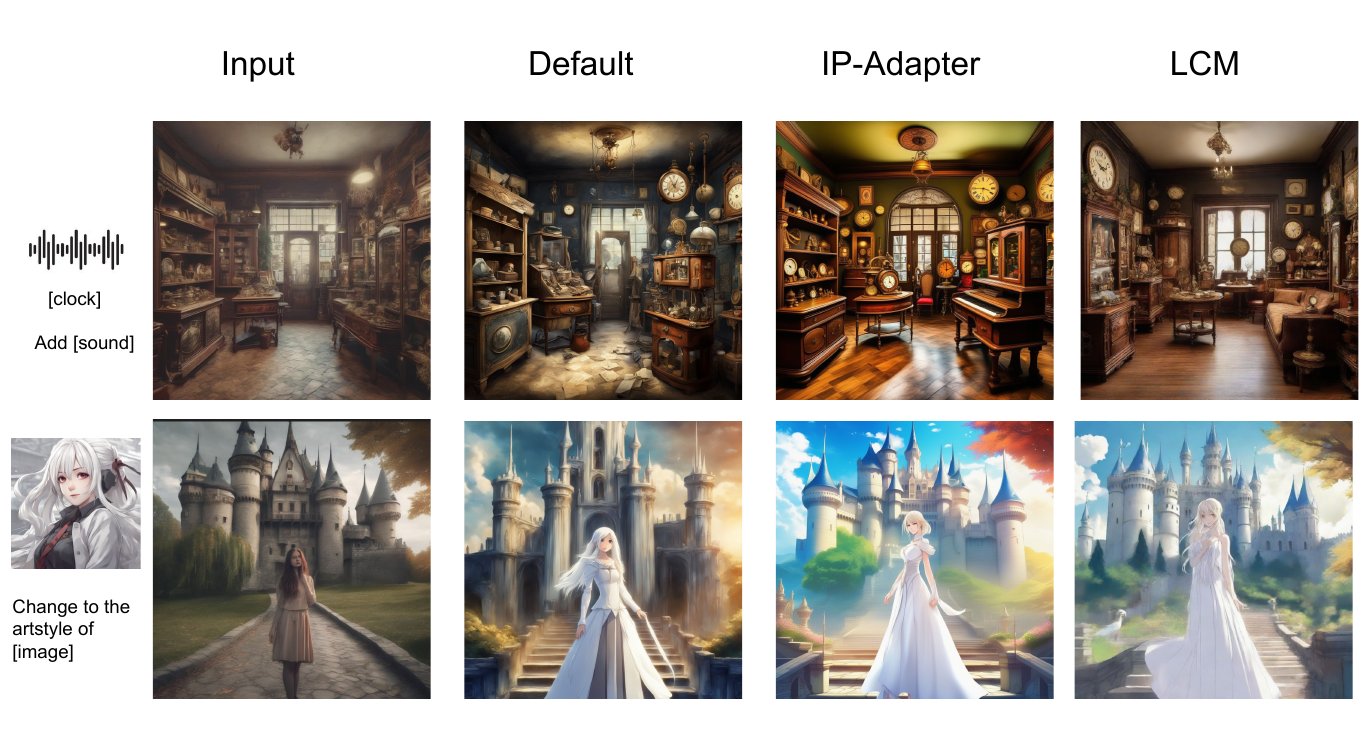}
    \caption{Qualitative Results of Swapping Diffusion Models. Because of our decoupled design, we can easily swap our diffusion model without retraining any other modules. The default model is a fine-tuned SDXL.  }
    \label{fig:additional_demo_ip}
\end{figure*}

\begin{figure*}[t]
    \centering
    \includegraphics[width=400px]{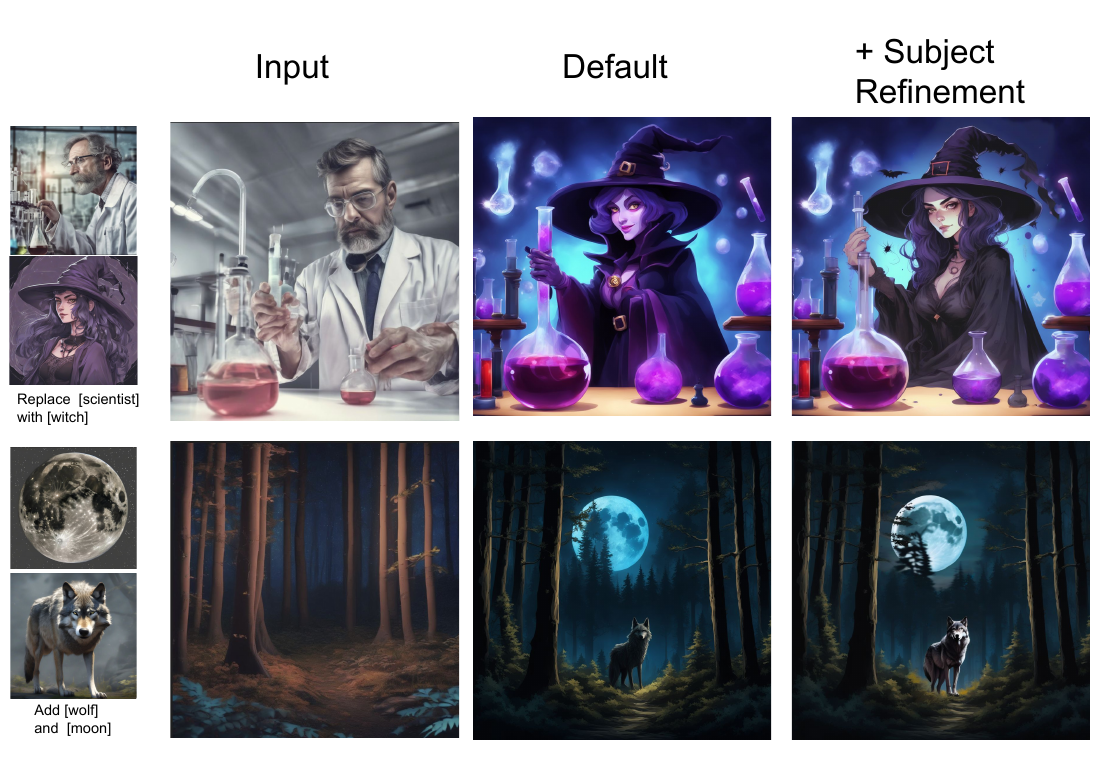}
    \caption{Qualitative Results of subject consistency refinement. With an additional subject refinement step, \ours can generate images that faithfully respect the detials of multiple reference images.  }
    \label{fig:subject}
\end{figure*}
\begin{figure*}[t]
    \centering
    \includegraphics[width=460px]{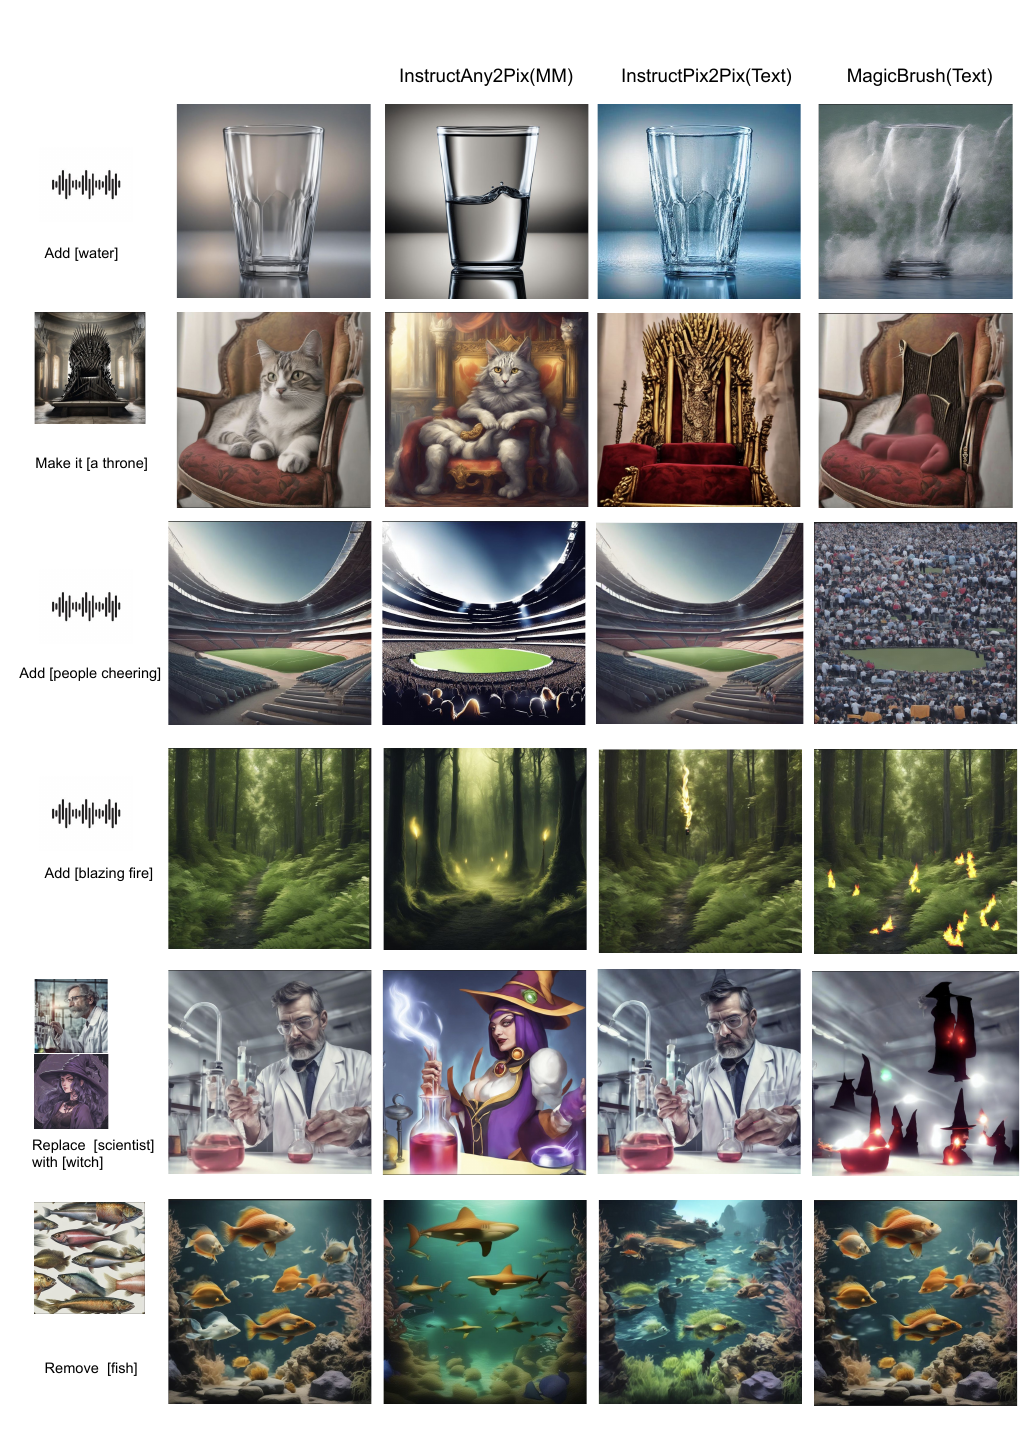}
    \caption{Qualitative Comparison against Magic Brush on MM-Inst dataset. Source and reference images are generated using SDXL \cite{podell2023sdxl}. Reference sound is generated using AudioLDM2 \cite{liu2023audioldm2}.}
    \label{fig:additional_demo2}
\end{figure*}

\begin{figure*}[t]
    \centering
    \includegraphics[width=440px]{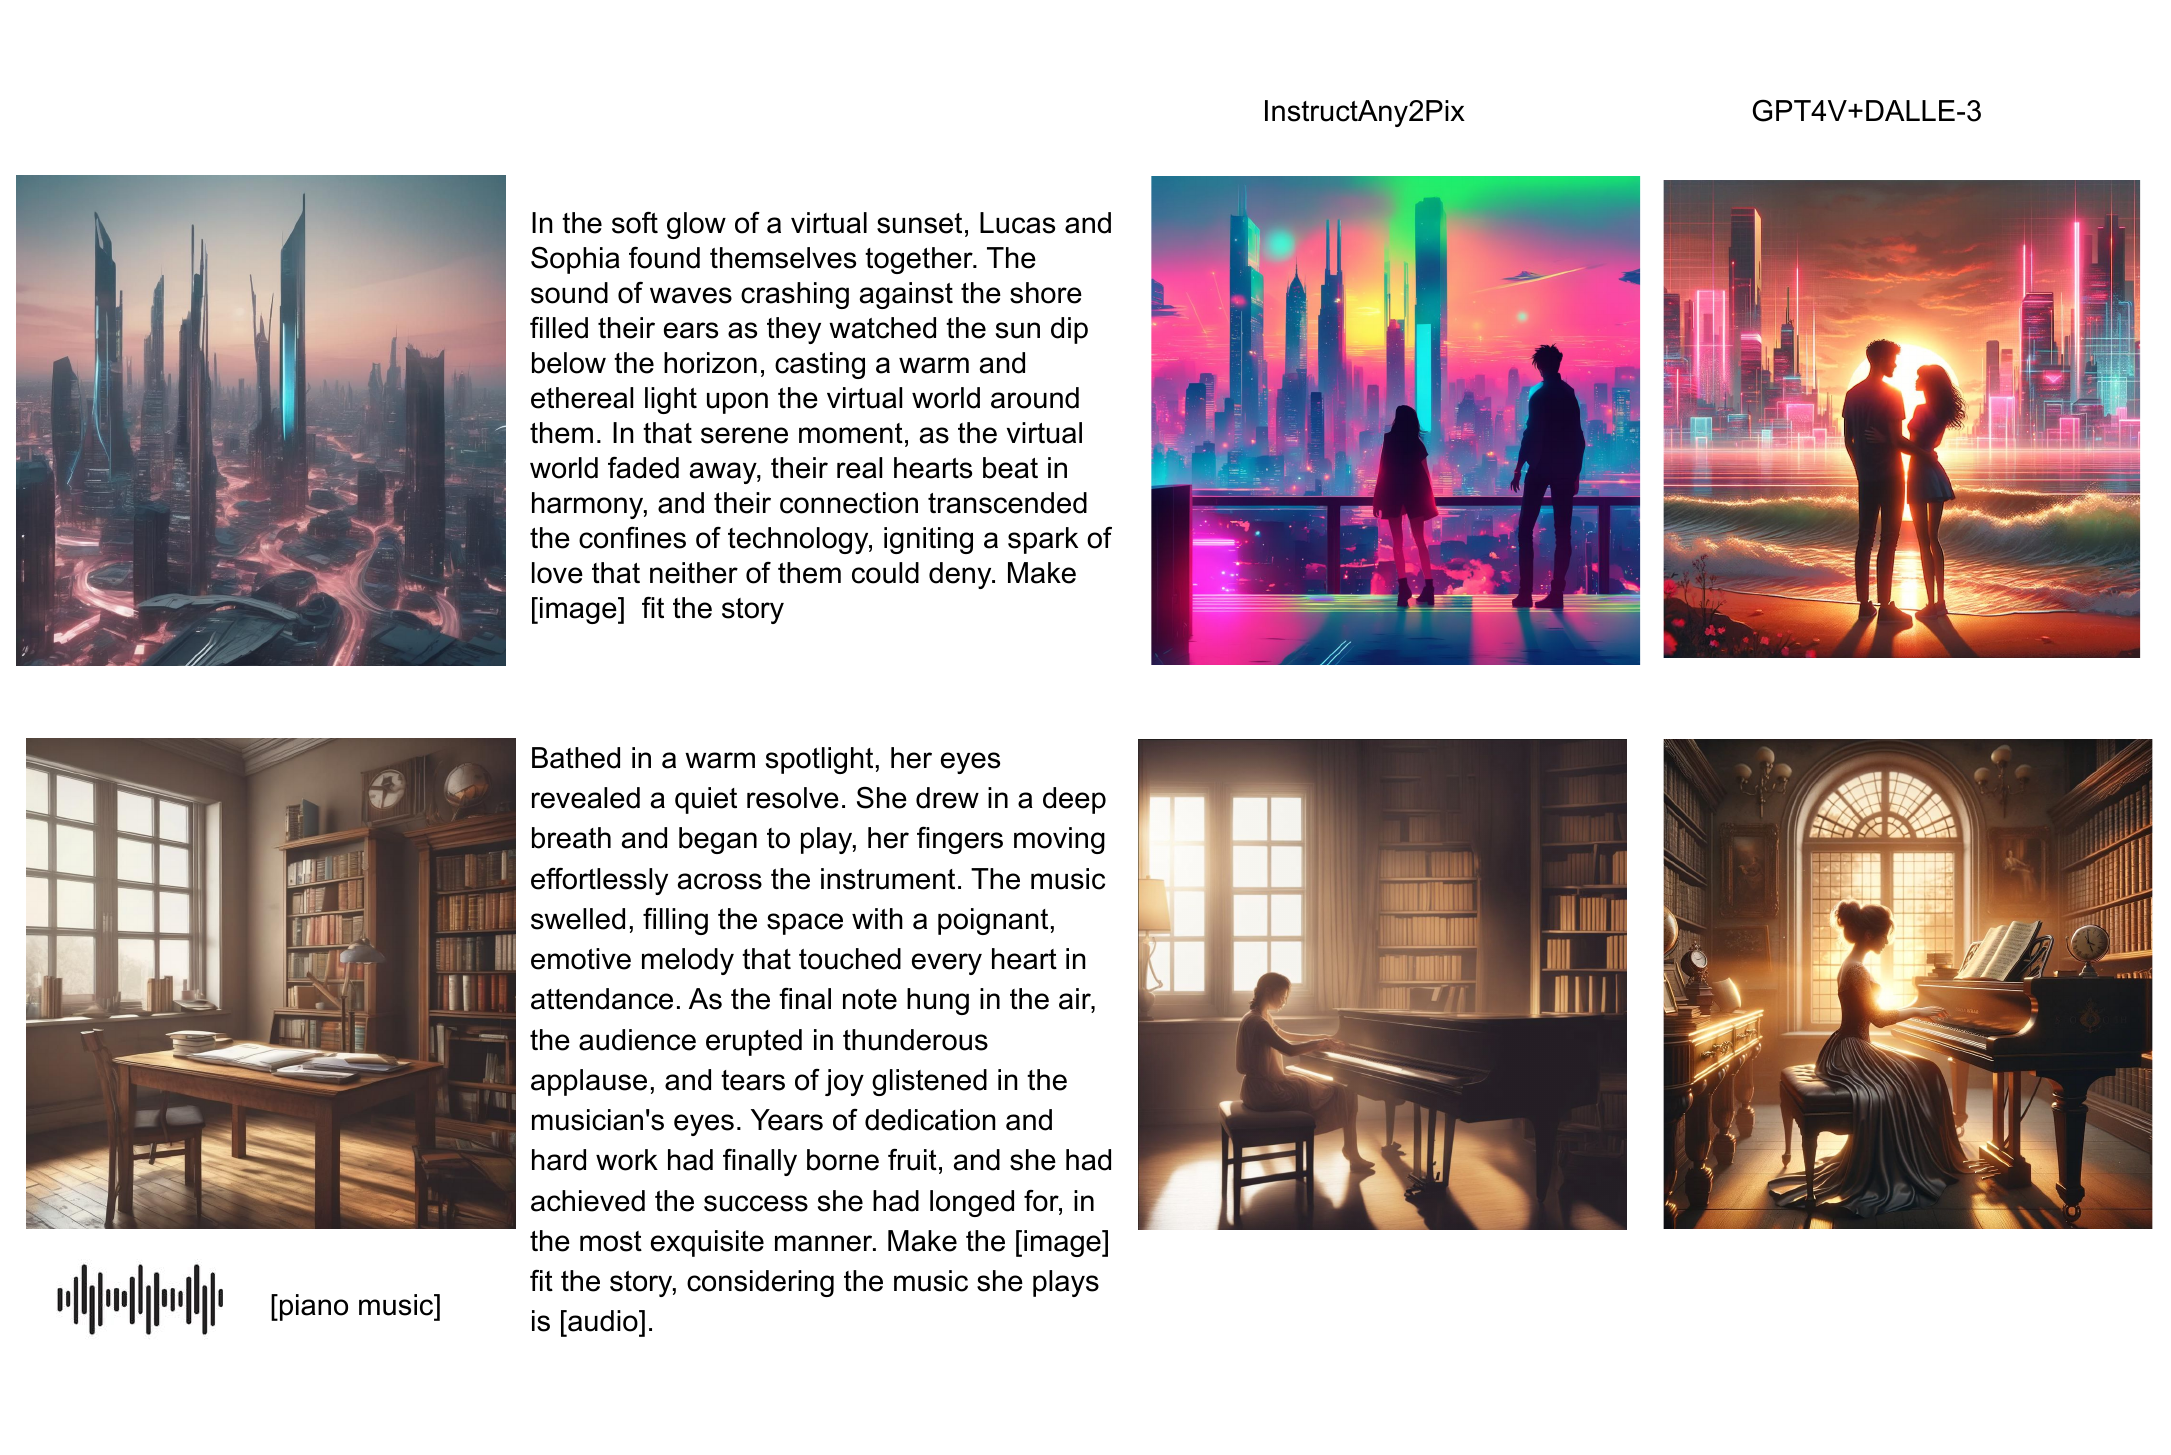}
    \caption{Generalizing to unseen instructions. We provide qualitative results on  extending \ours{} to unseen instructions. In particular, we test it on long-context story telling. We also provide comparisons with state-of-the-art model (GPT4V+DALLE-3)\cite{dalle3}. Considering the difference in model size and training data, \ours{} achieves impressive performance. In the first example, it was able to reason on the context of the love story and decide to add a couple to the image without explicitly instructed to do so. In the second example, it was able to extract supplementary information from audio that the ``instrument" referred in the passage is a piano. Since GPT4V cannot process audio, we reveal the anser in text for it. }
    \label{fig:generalization}
\end{figure*}

\begin{figure*}[h]
    \centering
    \includegraphics[width=460px]{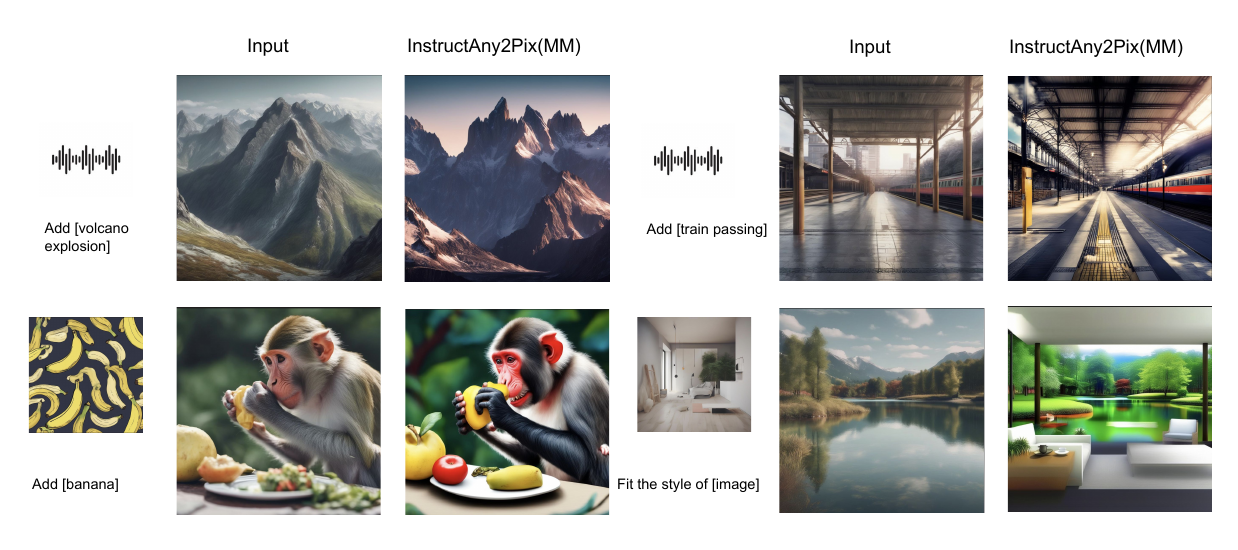}
    \caption{Failure Cases. (1) The sound of a volcano explosion is ambiguous and hard to distinguish. (2) Fails to add another passing train when there is already a train in the scene. (3) Fails to edit small details because of limitations in the training recipe. (4) Fails to perform style transfer when the intended style transfer is not intuitive, e.g., fitting a scenery to an interior design. In this example, the content of the reference image is used in lieu of the style. }
    \label{fig:additional_demo3}
\end{figure*}

\subsection{Diffusion Model}
We use the typical SDXL \cite{podell2023sdxl} implementation, which was originally conditioned on CLIP-ViT-G and CLIP-ViT-L text features. To avoid retraining cross-attention layers from scratch, we adopted an MLP projector that maps ImageBind features to the dimension of the original SDXL conditional inputs.

\subsection{Prior}
We adopted a decoder-only transformer. In particular, we followed the design of GPT-2 \cite{gpt2}. We substituted the token embedding layer with an MLP projector that maps ImageBind features to the hidden dimension of the transformer. We briefly explored using the instruction-following LLM (Vicuna-7B) \cite{vicuna}, but this proved infeasible because of slow training and convergence. We also briefly explored using a diffusion prior similar to that of DALLE-2\cite{ramesh2022}. In this setup the prior model predicts the the noise added to the target feature given a noised version of the target feature and time embedding. We observe no significant difference in generation quality and did not adopt this approach in our final method because of slower inference (20x).

\subsection{LLM}
In addition to architecture changes described in Section \ref{sec:method_llm}, we employed a two-stage training strategy to balance computation cost and convergence speed. During the first stage, we froze the LLM and only updated the projectors, input layers, and output layers. In the second stage, we updated all layers jointly. Using 8 Nvidia A6000 GPUs, the first stage training takes less than two days, while the second stage training takes less than four days.

\section{Additional Results}
In this section, we provide additional qualitative results to highlight the capability of \ours.

\subsection{Additional Editing Results}
In Figure \ref{fig:additional_demo} and \ref{fig:additional_demo_11}, we show more results across a broad spectrum of editing instructions, including adding and removing objects, multi-object scene composition, image style transfer, and fitting an image to the atmosphere of audio. These results complement Figures \ref{fig:multiturn}, \ref{fig:teaser}, \ref{fig:instructpix2pix}, \ref{fig:t2i}. They demonstrate our model's capability of understanding and performing a diverse set of instructions involving multi-modal inputs.

% For better viewing experiences, we also publish some of the demos to an anonymous website with playable audio included. The website is available at \href{https://sites.google.com/view/instructany2pix/project-page}{https://sites.google.com/view/instructany2pix/project-page}.

\subsection{Comparison with Text-Only Methods}
Since no previous work can perform image editing given multi-modal instructions, we provide a qualitative comparison with methods using text instructions. We compare our results against InstructPix2Pix \cite{brooks2023instructpix2pix} and MagicBrush \cite{Zhang2023MagicBrush} in Figure \ref{fig:additional_demo2}. For text-only methods, we convert the multi-modal instructions to equivalent text-only instructions. These results show that our model performs competitively against text-only methods, if not better. It also highlights some of the biases of our model. In particular, our model is biased towards artistic/painting output. This is likely caused by the biases of our dataset and training process. We provide further discussions in Section \ref{sec:appendix_limitations}.

\subsection{Generalizing to Longer Context}
Because \ours{} leverages the reasoning capability of a LLM, it has the potential to generalize to unseen instructions of a much longer context. To test this capability, we prompt the model to perform image edits based on a piece of story consisting of multiple sentences. This type of instruction is not included in our dataset. Additionally, the context-length is much longer than instructions in our dataset. \cref{fig:generalization} show these results. We also provide qualitative comparison against state-of-the are model (GPT4V+DALLE-3) \cite{dalle3}. Since GPT4V cannot understand audio inputs, we provide descriptions of audio in text. While GPT4V+DALLE-3 system cannot perform image edits, it can still generate an image based on textual and visual inputs. Considering the difference in model size and training data, \ours{} achieves impressive performance.

\subsection{Modularity}

Unlike existing end-to-end instruction-tuned models such as \cite{brooks2023instructpix2pix}, we adopt CLIP-ViT embeddings as a frozen, universal interface. This decoupled design allows us to swap our diffusion model without retraining any other parts, as long as the swapped model is also conditioned on CLIP-ViT embeddings. We highlight this capability in \cref{fig:additional_demo_ip}. We can easily swap the simple, fine-tuned SDXL with more complex image-conditioned adaptors such as IP-Adapter \cite{ye2023ip}, as well as different classes of generative models such as the Latent Consistency Model (LCM) \cite{luo2023latent}.

\subsection{Subject Consistency Refinement}

Subject consistency measures how well the generated images faithfully respect the objects in the reference image. For example, when trying to add a dog to an image, subject consistency measures the visual similarity of the added dog to the reference dog in various aspects, such as hair color, breed, and size. We can improve the subject consistency of \ours\ by training on additional data and modifying the model generation process.

In the subject consistency training process, the LLM is trained to output more than one [base] token. In addition to the standard [base] token, it also generates a list of edited objects and corresponding [base] tokens. These tokens are then used to retrieve reference images for the generation process. Finally, the diffusion model generates the edited images conditioned on these retrieved images.

Because fine-tuning a separate diffusion model that takes multiple image conditioning can be expensive, we adopt an iterative refinement process using our existing single-image-conditioned diffusion model. We first generate an image without any subject conditioning. Then, we find the corresponding segmentation mask of each subject in the object list generated by the LLM using an open-vocabulary segmentation model \cite{liu2023grounding, kirillov2023segany}. Finally, we perform masked image inpainting using our existing single-image-conditioned diffusion model on each of the subjects.

We provide qualitative results in Figure \ref{fig:subject}. The results show that with this subject refinement step, \textit{ours} can perform image editing that respects both the source image and reference images.

% Unlike existing end-to-end instruction-tuned models such as \cite{brooks2023instructpix2pix}, we adopt CLIP-ViT embeddings as a frozen, universal interface. This decoupled design allows us to swap our diffusion model without retraining any other parts, as long as the swapped model is also conditioned on CLIP-ViT embeddings. We highlight this capability in \cref{fig:additional_demo_ip}. We can easily swap the simple, fine-tuned SDXL with more complex image-conditioned adaptors such as IP-Adapter \cite{ye2023ip}, as well as different classes of generative models such as the Latent Consistency Model (LCM) \cite{luo2023latent}.

\section{Failure Cases}
We show some failure cases in Figure \ref{fig:additional_demo3}. Our method fails when the sound is rare, ambiguous, or hard to distinguish. For example, it fails to add a volcano explosion to an image of mountain ranges given the sound of a volcano explosion. It also cannot perform counting properly. For example, it fails to add another passing train to an image already with a train in it. This is likely caused by the inherent limitation of DDIM-inversion, which cannot perform fine-grained image editing operations. Additionally, our model may fail to perform style transfer on unconventional pairs. For example, when trying to fit a scenery to the style of minimalist interior design, it adds minimalist furniture to the scene.

\section{ Limitations and Future works}
\label{sec:appendix_limitations}
\subsection{Pretraining Data}
Our model makes use of pretrained a diffusion model \cite{podell2023sdxl} and LLM \cite{vicuna}. Hence, it may inherit biases from the training process of these models.

\subsection{Generation style}
Our model tends to bias towards artistic/painting outputs instead of photorealistic ones. This is caused by multiple factors: First, the LAION-Aesthetic-3M \cite{schuhmann2022laion} dataset used to recondition the diffusion model contains a lot of art and paintings. Additionally, LAION Aesthetic score used to condition the prior model is biased towards high saturation and artistic outputs. Lastly, we use SDXL to generate images for the MM-Inst dataset based on captions. Without explicit style keywords in prompts, we find that SDXL generations are biased towards artistic outputs as well. We will try addressing this limitation by exploring alternative ways of curating a high-quality dataset and explicitly adding diverse style prompts in the generation process.

\subsection{Fine-grained editing}
Our model fails to perform fine-grained image edits such as counting or editing a small part of an object (e.g., changing the traffic light to green). This is the inherent limitation of DDIM.

% 

% Because of the prohibitive computation cost, we leave customization for future exploration.

Since we use a single, multi-modal-aligned embedding to represent each input image, our model currently does not support instructions involving non-natural images and fine-grained spatial conditioning, e.g., ``make the [image] follow this [segmentation map]" or ``fit the [depth map] to image". However, in principle, it is possible to integrate existing conditioning adapters such as T2I~\cite{mou2023t2i} to our diffusion model and support these extra conditioning factors. 
We leave such explorations to future work.

\subsection{Reconstruction v.s. instructability tradeoff}
We observe that there is a trade-off between respecting user instructions and respecting  source images. This tradeoff also exists in previous works. Similar to InstructPix2Pix\cite{brooks2023instructpix2pix}, we introduce hyper-parameters that gives user control over how much should the output follow the source image ( \cref{fig:control}). In general, our model may introduce minor unintended changes to the image  since we do not directly fine-tune the diffusion model on image-editing. With improvements in base modality-specific models, we expect these issues to be mitigated even in the multimodal setting.

% \subsection{Incorporating extra conditions (e.g. depth map)}
% Because we use a single, multi-modal-aligned embedding to represent each input image, our model currently does not support instructions involving non-natural images and fine-grained spatial conditioning, e.g., ``make the [image] follow this [segmentation map]" or ``fit the [depth map] to image". However, in principle, it is possible to integrate existing conditioning adapters such as T2I~\cite{mou2023t2i} to our diffusion model and support these extra conditioning factors. Due to the customizeft them for future works to explore.

In spite of these limitations, our model successfully extends the scope of image editing instructions to multi-modal, multi-object inputs while achieving a favorable balance between performance and computation cost. We hope future works will further scale our approach to diverse editing without incurring substantial computational overhead.
